# Supplementary material for: Reversible quantum information spreading in many-body systems near criticality
Source: arXiv:1812.09237 ancillary file (2019-09-17)
Supplement: Supplementary file 1 [file supplemental_material.pdf]

# Supplemental material for Reversible quantum information spreading in many-body systems near criticality

Quirin Hummel, Benjamin Geiger, Juan Diego Urbina, and Klaus Richter  
*Institut für Theoretische Physik, Universität Regensburg, D-93040 Regensburg, Germany*  
(Dated: September 16, 2019)

## Appendix A: The truncated model

The starting point is the Hamiltonian for bosons on a ring with attractive ( $\tilde{\alpha} \geq 0$ ) contact interaction formulated in second quantization [1]

$$\hat{H} = \int_0^{2\pi} d\theta \left[ -\hat{\psi}^\dagger(\theta) \partial_\theta^2 \hat{\psi}(\theta) - \frac{\pi \tilde{\alpha}}{2} \hat{\psi}^\dagger(\theta) \hat{\psi}^\dagger(\theta) \hat{\psi}(\theta) \hat{\psi}(\theta) \right], \quad (\text{A1})$$

where the field operators  $\hat{\psi}^\dagger(\theta)$  and  $\hat{\psi}(\theta)$  are creation and annihilation operators of bosons at position  $\theta$  with periodic identification  $\hat{\psi}(\theta + 2\pi) = \hat{\psi}(\theta)$  and obeying the bosonic commutation relations

$$\begin{aligned} [\hat{\psi}(\theta), \hat{\psi}(\theta')] &= [\hat{\psi}^\dagger(\theta), \hat{\psi}^\dagger(\theta')] = 0, \\ [\hat{\psi}(\theta), \hat{\psi}^\dagger(\theta')] &= \delta(\theta - \theta'), \end{aligned} \quad (\text{A2})$$

making use of the restriction of  $\theta$  to one specific interval of length  $2\pi$ . The form (A1) corresponds to the Lieb-Liniger model [2] when setting units by  $\frac{\hbar^2}{2m} = 1$  and  $L = 2\pi$ . In other words, energy will be given in units of

$$[E] = \frac{4\pi^2 \hbar^2}{2mL^2}, \quad (\text{A3})$$

where  $L$  is the length of the system. The coupling parameter is related to the two-body scattering length  $a_{3D}$  (which is negative for attractive interactions considered here) by [3]

$$\tilde{\alpha} = -\frac{2m}{\pi^2 \hbar} L a_{3D} \omega_\perp, \quad (\text{A4})$$

when applied to realistic ultracold quasi-1D Bose gases in the regime  $a_{3D} \ll \sqrt{\hbar/m\omega_\perp}$  of strong transversal confinement with trapping frequency  $\omega_\perp$ . Eq. (A1) also admits to account for confinement induced resonances [3] by a modification of (A4). We do not take into account effective three-body interaction due to finite confinement and the consequent existence of excited trimer states reported in [4–6].

By Fourier decomposition of the field operators into momentum modes

$$\hat{\psi}(\theta) = \frac{1}{\sqrt{2\pi}} \sum_{k \in \mathbb{Z}} e^{ik\theta} \hat{a}_k, \quad (\text{A5})$$

where the annihilation and creation operators in the momentum modes fulfill

$$\begin{aligned} [\hat{a}_k, \hat{a}_l] &= [\hat{a}_k^\dagger, \hat{a}_l^\dagger] = 0, \\ [\hat{a}_k, \hat{a}_l^\dagger] &= \delta_{kl}, \end{aligned} \quad (\text{A6})$$

and truncating the Hilbert space to the three lowest single particle momentum modes  $k = -1, 0, 1$ , or, equivalently, neglecting the occupation of higher modes  $|k| \geq 2$  by setting them to zero, yields

$$\hat{H}_3 = \sum_{k=-1}^1 k^2 \hat{a}_k^\dagger \hat{a}_k - \frac{\tilde{\alpha}}{4} \sum_{k,l,m,n=-1}^1 \delta_{k+l,m+n} \hat{a}_k^\dagger \hat{a}_l^\dagger \hat{a}_m \hat{a}_n. \quad (\text{A7})$$

The validity of this truncation comes from the relevance of low momentum modes for the quantum phase transition [7–9] and goes far beyond a perturbative expansion in powers of  $\tilde{\alpha}$ . One can easily show that

$$\begin{aligned} [\hat{H}_3, \hat{N}] &= 0, \\ [\hat{H}_3, \hat{K}] &= 0, \end{aligned} \quad (\text{A8})$$

with the total number of particles and momentum operator

$$\begin{aligned} \hat{N} &= \sum_{k \in \{-1,0,1\}} \hat{a}_k^\dagger \hat{a}_k, \\ \hat{K} &= \sum_{k \in \{-1,0,1\}} k \hat{a}_k^\dagger \hat{a}_k = \hat{a}_1^\dagger \hat{a}_1 - \hat{a}_{-1}^\dagger \hat{a}_{-1}. \end{aligned} \quad (\text{A9})$$

When a specific quantum state is considered, an indicator for the defect introduced due to the truncation (A7) is the depopulation of the single-particle ground state  $k = 0$ . If an eigenstate of (A7) in the truncated Hilbert space is merely slightly populated in the modes  $k = \pm 1$ , one can assume that the occupation of all truncated modes  $|k| > 1$  in the corresponding exact eigenstate of the full Hamiltonian is even smaller and thus negligible. As concerns the QPT and the excited state QPT (ESQPT) relevant for scrambling and dynamics of inter-particle correlations, the depletion of the condensate can be made arbitrarily small by increasing the number of particles, which allows to reduce  $N\tilde{\alpha}$  arbitrarily close to the MF critical value of 1 and still stay in a sufficiently supercritical regime to fulfill all requirements necessary for the analysis.

## Appendix B: The classical limit

In order to obtain the classical counterpart of the truncated quantum system, one has to replace the creation and annihilation operators by complex valued classical

variables

$$\begin{aligned}\hat{a}_k &\mapsto \phi_k =: \frac{1}{\sqrt{2}}(q_k + ip_k), \\ \hat{a}_k^\dagger &\mapsto \phi_k^* =: \frac{1}{\sqrt{2}}(q_k - ip_k),\end{aligned}\quad (\text{B1})$$

with the new classical coordinates  $q_k$  and canonically conjugated momenta  $p_k$  that take real values. In addition special care has to be taken considering the ordering of operators. The correct prescription [10] thereby is to replace symmetrically ordered products of operators

$$\left\{ \hat{a}_{k_1} \cdots \hat{a}_{k_m} \hat{a}_{l_1}^\dagger \cdots \hat{a}_{l_n}^\dagger \right\}_{\text{sym}} \mapsto \phi_{k_1} \cdots \phi_{k_m} \phi_{l_1}^* \cdots \phi_{l_n}^*, \quad (\text{B2})$$

where the symmetric ordering is defined by the sum of all possible orderings divided by their number

$$\{\hat{c}_1 \cdots \hat{c}_n\}_{\text{sym}} := \frac{1}{n!} \sum_{\sigma \in S_n} \hat{c}_{\sigma(1)} \cdots \hat{c}_{\sigma(n)}, \quad (\text{B3})$$

where the  $c_j$  can be any creation and/or annihilation operators and  $\sigma$  runs over all permutations of  $n$  (summarized by the symmetric group  $S_n$ ). Ordering the operators in (A7) using (A6) and performing the prescription (B2) yields the classical Hamilton function for the truncated Lieb-Liniger model

$$\begin{aligned}H_{\text{cl}} &= \sum_k \left( k^2 + \frac{3\tilde{\alpha}}{2} \right) |\phi_k|^2 \\ &\quad - \frac{\tilde{\alpha}}{4} \sum_{k,l,m,n} \delta_{k+l,m+n} \phi_k^* \phi_l^* \phi_m \phi_n - \frac{9\tilde{\alpha}}{8} - 1,\end{aligned}\quad (\text{B4})$$

where the specification of the index sets in the sums has been omitted in order to ease notation.

The canonical transformation

$$\begin{aligned}\frac{1}{\sqrt{2}}(q_k + ip_k) &\mapsto \sqrt{n_k} e^{-i\vartheta_k} \\ n_k &\in \mathbb{R}^+, \vartheta_k \in [0, 2\pi)\end{aligned}\quad (\text{B5})$$

fulfills

$$\begin{aligned}\{\vartheta_k, \vartheta_l\}_{\mathbf{q}, \mathbf{p}} &= \{n_k, n_l\}_{\mathbf{q}, \mathbf{p}} = 0, \\ \{\vartheta_k, n_l\}_{\mathbf{q}, \mathbf{p}} &= \delta_{kl},\end{aligned}\quad (\text{B6})$$

with Poisson brackets

$$\{f, g\}_{\mathbf{q}, \mathbf{p}} := \sum_k \left( \frac{\partial f}{\partial q_k} \frac{\partial g}{\partial p_k} - \frac{\partial g}{\partial q_k} \frac{\partial f}{\partial p_k} \right). \quad (\text{B7})$$

Note that the transformation into polar coordinates (B5) introduces a punctuation of the  $(q_k, p_k)$ -planes, so that orbits or paths cannot continuously be deformed across these singularities using  $(\vartheta_k, n_k)$  coordinates. This is especially important for the calculation of Maslov indexes [11] needed for the EBK quantization of the model.

The transformation brings the Hamilton function into the form

$$\begin{aligned}H_{\text{cl}} &= \sum_k \left( k^2 + \frac{3\tilde{\alpha}}{2} \right) n_k - \frac{9\tilde{\alpha}}{8} - 1 - \frac{\tilde{\alpha}}{4} [n_0^2 + n_1^2 + n_{-1}^2 \\ &\quad + 4(n_0 n_1 + n_0 n_{-1} + n_1 n_{-1}) \\ &\quad + 4n_0 \sqrt{n_1 n_{-1}} \cos(2\vartheta_0 - \vartheta_1 - \vartheta_{-1})].\end{aligned}\quad (\text{B8})$$

In addition to energy conservation  $\frac{d}{dt} H_{\text{cl}} = \frac{\partial}{\partial t} H_{\text{cl}} = 0$  there exist two constants of motion

$$\tilde{N} = n_0 + n_{-1} + n_1, \quad (\text{B9})$$

$$\tilde{K} = n_1 - n_{-1},$$

$$\{\tilde{N}, H_{\text{cl}}\} = \{\tilde{K}, H_{\text{cl}}\} = 0, \quad (\text{B10})$$

closely related to the total number of particles  $N$  and the total momentum  $K$  as eigenvalues of (A9).

A further point transformation takes the phase space variables  $(\vartheta_0, \vartheta_{-1}, \vartheta_1, n_0, n_{-1}, n_1)$  into  $(\varphi, \varphi_N, \varphi_K, n_0, \tilde{N}, \tilde{K})$  given by

$$\begin{aligned}\varphi &= \vartheta_0 - \frac{1}{2}(\vartheta_1 + \vartheta_{-1}), \\ \varphi_N &= \frac{1}{2}(\vartheta_1 + \vartheta_{-1}), \\ \varphi_K &= \frac{1}{2}(\vartheta_1 - \vartheta_{-1}),\end{aligned}\quad (\text{B11})$$

leaving us with the expression [cf. Eq. (6) of the main text]

$$\frac{H_{\text{cl}}}{\tilde{N}} = \omega(\varphi, z, l) - \frac{\alpha}{4} - \frac{1}{\tilde{N}} + \frac{3\alpha}{2\tilde{N}} - \frac{9\alpha}{8\tilde{N}^2} \quad (\text{B12})$$

where the classical dynamics is completely determined by

$$\begin{aligned}\omega(\varphi, z, l) &= 1 - z - \frac{\alpha}{4} \left[ \frac{1}{2} + z - \frac{3}{2} z^2 - \frac{1}{2} l^2 \right. \\ &\quad \left. - 2z \sqrt{(1-z)^2 - l^2} (1 - 2 \cos^2 \varphi) \right].\end{aligned}\quad (\text{B13})$$

Here we used the scaled variables

$$z := \frac{n_0}{\tilde{N}}, \quad l := \frac{\tilde{K}}{\tilde{N}}, \quad \alpha := \tilde{\alpha} \tilde{N}, \quad (\text{B14})$$

where  $z$  is closely related to the classical version of the (subcritical) condensate fraction and  $l$  is closely related to the average angular momentum per particle. These two relations become exact in the limit  $N \rightarrow \infty$ . The dynamically constant energy shift in Eq. (B12) corresponds, up to  $\mathcal{O}(N^{-1})$ -corrections, to the MF ground state energy per particle  $-\tilde{\alpha}N/4$  one finds in the subcritical regime when solving the non-linear Schrödinger equation [1, 12] corresponding to the continuous model (A1).

As the scaled version (B13) does not depend on  $\tilde{N}$  anymore the influence of the number of bosons  $N$  on the physics will take place purely on the quantum level through its role as the effective quantum of action  $\hbar_{\text{eff}} = 1/\tilde{N}$  in Eq. (10) of the main text.

### Appendix C: Universal separatrix quantization

In general, we focus on critical systems with an essentially one-dimensional description. In particular this applies to integrable systems by fixing  $D - 1$  conserved quantities (like number of particles  $N$  and total momentum  $K$  in the truncated model considered in the main text), where  $D$  is the number of (collective) degrees of freedom. Nevertheless one can think of more general systems that become essentially one-dimensional around criticality whenever a clear scale separation allows for adiabatic treatment of additional degrees of freedom.

To be more specific, we focus on the supercritical regime and address local universal features in spectral and dynamical properties that are dominated by (highly) excited states close to transition. Whenever an ESQPT can be attributed to a separatrix crossing in the MF dynamics in effectively one dimension, which we consider as a generic mechanism for second order quantum phase transitions, a quantization condition similar to Eq. (10) of the main text applies in the semiclassical picture. For this we consider orbits on both sides close to a separatrix which translates to quantum states close to criticality for large  $N$  (small  $\hbar_{\text{eff}}$ ) while fixing the external parameter that drives the transition.

Although we are eventually interested in the application to critical MB systems, the following analysis is not restricted to this interpretation. Therefore we consider here any one-dimensional quantum system that derives from a quantization of a classical Hamiltonian system with a separatrix structure and write standard commutation relations as  $[\hat{p}, \hat{q}] = -i\hbar$ , which defines the meaning of  $\hbar$  in a specific context. While  $\hbar$  can be the actual Planck constant, it has to be reinterpreted as *effective* quantum of action  $\hbar_{\text{eff}} \sim 1/N$  in the special case of MB systems, with MF dynamics formally defining the corresponding classical analogue.

For simplicity we set the classical energy, i.e., the Hamilton function  $\omega(q, p)$ , to  $\omega = 0$  directly on the separatrix. In the limit  $\hbar \rightarrow 0$  (or  $N \rightarrow \infty$  in the MB context) the quantized energy levels close to  $\omega = 0$  get arbitrarily small, allowing to use a specific local expansion of the Hamilton function  $\omega(q, p)$  around the separatrix to determine the corresponding classical orbits. For this one has to realize that  $\omega$  is quadratic at the saddle points where the separatrix intersects itself while it behaves only linearly on other parts of the separatrix. We thus split the corresponding action integrals into local parts close to the saddle points using a quadratic expansion there and non-local parts using linearization around the separatrix otherwise. The orbit actions (when defined relative to the separatrix) are dominated by the local regions around the hyperbolic fixed points while non-local parts of the separatrix give sub-dominant corrections as illustrated in Fig. C1 for the case of the specific model studied in the main text.

Consequently, a subsequent general semiclassical analysis reveals that the quantized levels close to  $\omega = 0$

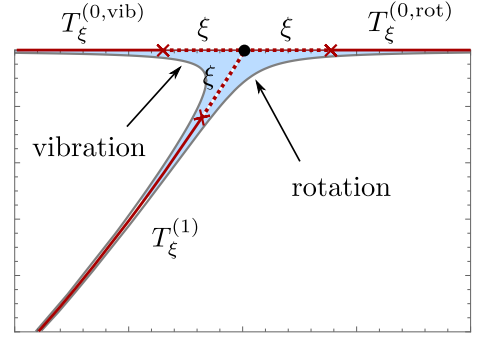

FIG. C1. Two orbits very close to the separatrix in energy. The corresponding orbit actions are dominated by the region around the saddle point (areas shown in light blue). Sub-dominant non-local contributions are given by on-separatrix traversal times  $T_\xi^{(0,rot)}$ ,  $T_\xi^{(0,vib)}$  and  $T_\xi^{(1)}$  cut off at distances  $\xi$  from the hyperbolic fixed point.

depend only on properties of the saddle point and the separatrix itself. We focus here on the case where the parameters characterizing the orbits on both sides of the separatrix are the same, which is the case in the 3-mode model at hand. The generalization to arbitrary situations is straightforward [11]. We find general formulas for semiclassical separatrix quantization, in the simplest form expressed as the smooth density of states

$$\bar{\rho}(\omega) = -\frac{1}{2\pi\hbar} \frac{1}{\lambda} \log \frac{|\omega|}{\Omega} + \frac{t_{\text{sep}}}{2\pi\hbar} + \mathcal{O}(\omega). \quad (\text{C1})$$

The discrete energy levels obtained by semiclassical action quantization around the ESQPT are [see Eq. (10) of the main text]

$$\omega_{[k]} \approx \frac{-2\pi\hbar\lambda(\mu + k)}{\mathcal{W}_{-1}(-2\pi\hbar\lambda\Omega^{-1}e^{-1-\lambda t_{\text{sep}}}|\mu + k|)}, \quad k \in \mathbb{Z}, \quad (\text{C2})$$

ordered by  $k$  and with  $\omega_{[0]}$  referring to the first level lying above the separatrix energy  $\omega = 0$ . In (C1) and (C2),  $\mathcal{W}_{-1}$  is the lower branch of the Lambert- $\mathcal{W}$  function, which is the solution to  $\mathcal{W}(x)e^{\mathcal{W}(x)} = x$  with  $x \in [-e^{-1}, 0[$  and  $\mathcal{W}_{-1}(x) \leq -1$  [13]. The inverse total stability exponent  $\lambda^{-1} = \sum_j 1/\lambda^{(j)}$  is the sum of reciprocal stability exponents of all saddle points  $j$  involved, while the constant index shifts  $\mu \in [0, 1[$  are related to the Maslov index and separatrix action. We introduced a typical classical (i.e., independent of  $\hbar$ ) unit of energy  $\Omega$  that characterizes the breakdown of the involved expansions of the classical Hamilton function. As a local approximation, Eq. (C2) is valid as long as  $\omega_{[k]}/\Omega \ll 1$ . The expressions (C1) and (C2) finally do not depend on the specific choice of  $\Omega$  as the regularized separatrix traversal time  $t_{\text{sep}}$  is given by

$$t_{\text{sep}} = T^{\text{conv}} - \sum_j \frac{1}{\lambda^{(j)}} \log \left( \frac{\Omega}{2} \left( \frac{1}{\lambda_+^{(j)}} + \frac{1}{|\lambda_-^{(j)}|} \right) \right), \quad (\text{C3})$$

where  $\lambda_\pm^{(j)}$  are the positive and negative eigenvalues of the Hessian when expanding the Hamiltonian around the

saddle point  $j$  and

$$T^{\text{conv}} := \lim_{\xi \rightarrow 0} \left( T_\xi + \frac{2}{\lambda} \log \xi \right) \quad (\text{C4})$$

is the convergent part of the separatrix traversal time, with  $T_\xi$  the sum of on-separatrix traversal times cut off at (phase-space-) distances  $\xi$  from all involved saddle points. To calculate the non-local constant  $t_{\text{sep}}$  in a specific system one has to give meaning to  $\lambda_\pm$  and phase space distance  $\xi$ , which are actually ill-defined objects because in general a phase space in Hamiltonian mechanics does not have a metric but rather a symplectic form (Note that in contrast,  $\lambda$  is well defined). To do the calculation one has to define arbitrary units  $q_0$  of length and  $p_0$  of momentum to get a dimensionless phase-space. The meaning of  $\lambda_\pm$  and  $\xi$  are then defined in that space (using Euclidean norm) with the outcome  $t_{\text{sep}}$  not depending on the particular choice of  $q_0$  and  $p_0$ .

The dominant term  $\sim \log |\omega|$  in Eq. (C1) determined locally by only the saddle point has been found before (see [14] for a corresponding classification of ESQPTs) by counting the reduction of classical phase space volumes due to potential energy maxima. In contrast, the subdominant terms, non-locally determined by properties of the whole separatrix, are, to the best of our knowledge, original. More importantly, the discrete levels (C2) not only describe the local spectrum on average, as given by Eq. (C1). Equation (C2) may indeed be obtained from Eq. (C1) by effective quantization  $\int_{0+}^{\omega[k]} d\omega \bar{\rho}(\omega) = \mu + k$  of the average density of states. Moreover, the form (C2) has been noted [15] in a corresponding analysis. However, in the analysis presented here it represents by no means just an artificially constructed, maximally uniform spectrum consistent with  $\bar{\rho}$ . Instead, Eq. (C2) gives the actual individual levels obtained by applying the full semiclassical quantization condition as in Eq. (10) of the main text, as long as  $\omega[k]/\Omega \ll 1$ . The local spectrum thus is indeed as uniform as possible, absent of any fluctuations. This is due to the one-dimensional description and has the far reaching consequence of asymptotically constant level spacing (see Appendix E).

#### Appendix D: Separatrix quantization in the model

Using the scaled phase space variables [Eq. (8) of the main text] and scaled Hamiltonian (energy per particle)  $\omega(z, \varphi)$  [Eq. (7) of the main text] gives the Hessian

$$\mathcal{H} = \begin{pmatrix} 0 & -2\sqrt{\alpha-1} \\ -2\sqrt{\alpha-1} & 2 - \frac{\alpha}{4} \end{pmatrix} \quad (\text{D1})$$

at the hyperbolic fixed point (here chosen to be the one located at  $\varphi > 0$ ). Due to symmetry the corresponding stability exponent  $\lambda^{(j)} = \sqrt{-\det \mathcal{H}} = 2\sqrt{\alpha-1}$  is the same for both fixed points  $j = 1, 2$ . The total exponent determining the dominant spacing [see Eq. (11) of the

main text] is therefore

$$\lambda = \sqrt{\alpha-1}, \quad (\text{D2})$$

while for the subdominant contribution  $t_{\text{sep}}$  the eigenvalues of  $\mathcal{H}$  give

$$\frac{1}{2} \left( \frac{1}{\lambda_+^{(j)}} + \frac{1}{|\lambda_-^{(j)}|} \right) = \frac{\sqrt{(1 - \frac{\alpha}{8})^2 + 4(\alpha-1)}}{4(\alpha-1)}. \quad (\text{D3})$$

For the separatrix traversal times the separatrix can be split into three segments with a cutoff at distance  $\xi$  from the fixed points (see Fig. C1), defining the traversal times *i*)  $T_\xi^{(0, \text{rot})}$  for the outer upper boundary at  $\cos^2 \varphi < 1/\alpha$  for rotations, *ii*)  $T_\xi^{(0, \text{vib})}$  for the inner upper boundary at  $\cos^2 \varphi > 1/\alpha$  for vibrations and *iii*)  $T_\xi^{(1)}$  for the curved separatrix segment between the two saddle points separating vibrations and rotations. We calculate the traversal times as

$$T_\xi^{(\gamma)} = \int_{\mathcal{C}_\gamma} d\varphi \left| \frac{\partial \omega}{\partial z} \right|_{\mathcal{C}_\gamma}^{-1} \quad (\text{D4})$$

along the corresponding segment  $\mathcal{C}_\gamma$ . Elementary integration then yields

$$T_\xi^{(\gamma)} = -\frac{1}{\sqrt{\alpha-1}} \log \xi + T_{\text{conv}}^{(\gamma)} + \mathcal{O}(\xi), \quad (\text{D5})$$

with the convergent parts on the respective segments

$$T_{\text{conv}}^{(0, \text{rot})} = T_{\text{conv}}^{(0, \text{vib})} = \frac{1}{\sqrt{\alpha-1}} \log \left( \frac{2}{\alpha} \sqrt{\alpha-1} \right), \quad (\text{D6})$$

$$T_{\text{conv}}^{(1)} = T_{\text{conv}}^{(0, \text{rot})} + \frac{1}{\sqrt{\alpha-1}} \log \sqrt{1 + \left( \frac{\partial z^{\text{sep}}}{\partial \varphi} \right)_{\text{FP}}}. \quad (\text{D7})$$

The second term in (D7) essentially compensates (D3) in the total regularized separatrix traversal time (C3) and may be associated with the specific choice of phase space coordinates and Euclidean norm that drops out eventually. Finally, the regularized separatrix traversal time (C3) reads (setting  $\Omega = 1$ )

$$t_{\text{sep}} = \frac{1}{\sqrt{\alpha-1}} \log \left( \frac{128(\alpha-1)^2}{\alpha^2(8-\alpha)} \right) \quad (\text{D8})$$

on both sides of the transition.

Altogether, combining (C1), (D2) and (D8), the asymptotic DoS  $\bar{\rho}(E) = \bar{\rho}(\omega)/\tilde{N}$  close to the ESQPT is given by [see Eq. (11) of the main text]

$$\bar{\rho}(E) = \frac{-1}{2\pi\lambda} \log \left( \frac{|E - E_{\text{sep}}|}{\tilde{N}} \right) + \frac{t_{\text{sep}}}{2\pi} + \mathcal{O} \left( \frac{E - E_{\text{sep}}}{N^2} \right). \quad (\text{D9})$$

Similarly, the application of Eq. C2 with  $\hbar_{\text{eff}} = 1/\tilde{N}$  yields

$$E_{[k]} \approx \frac{-2\pi\lambda(\mu + k)}{\mathcal{W}_{-1} \left( -2\pi\lambda/\tilde{N} e^{-1-\lambda t_{\text{sep}}} |\mu + k| \right)}, \quad k \in \mathbb{Z}. \quad (\text{D10})$$

### Appendix E: Asymptotic spectral equidistance

Considering the formal semiclassical limit  $\hbar \rightarrow 0$  in (C2) by application of the asymptotics  $\mathcal{W}_{-1}(x) = \log(-x) - \log(-\log(-x)) + \mathcal{O}[\log(-\log(-x))/\log(-x)]$  results in the universal asymptotic law

$$\omega_{[k]} \sim 2\pi\hbar\lambda_\sigma \left(\log \frac{s_0}{\hbar}\right)^{-1} (\mu_\sigma + k) \times \left(1 + \mathcal{O}\left(\frac{\log \log \frac{s_0}{\hbar}}{\log \frac{s_0}{\hbar}}\right)\right) \quad (\text{E1})$$

of constant level spacing that depends only on the stability exponents associated with involved saddle-points. Here,  $s_0$  is an arbitrarily chosen but classically defined (typical) action of the system, merely introduced to maintain proper units while asymptotically irrelevant.

If  $\lambda_< = \lambda_> \equiv \lambda$  the asymptotic level spacing (E1) induces the single Ehrenfest-like time scale [see Eq. (12) of the main text]

$$\tau \sim \frac{1}{\lambda} \log \frac{s_0}{\hbar} \quad (\text{E2})$$

for quantum mechanical processes that dominantly involve the states in the band of high DoS around the separatrix energy  $\omega = 0$ .

There is, however, a subtle constraint involved in the asymptotic expressions (E1) and (E2), for which the quantum number  $k$  was assumed to be fixed during the limiting process. For a dynamical process, however, typically the number of dominantly involved states also grows with  $s_0/\hbar$ . Therefore one has to address the question of how many states around the separatrix, as a function of  $\hbar$ , can be considered asymptotically equidistant. Let  $K = K(\hbar)$  denote this number. We presume  $\lim_{\hbar \rightarrow 0} \hbar K(\hbar) = 0$ , as implied by the prerequisite  $\lim_{\hbar \rightarrow 0} \omega_{[K(\hbar)]} = 0$  necessary for the close-to-separatrix quantization (C1) and (C2). As indicator for equidistance we consider the mean level spacing  $\langle \Delta\omega \rangle_K = \omega_{[K]}/K$  averaged over  $K(\hbar)$  states lying around  $\omega = 0$ . Based on (C2) the asymptotics for  $\mathcal{W}_{-1}$  give

$$\langle \Delta\omega \rangle_K = \frac{2\pi\hbar\lambda}{\log \frac{s_0}{\hbar} - \log K(\hbar)} \times \left(1 + \mathcal{O}\left(\frac{\log \log \frac{s_0}{\hbar K}}{\log \frac{s_0}{\hbar K}}\right)\right). \quad (\text{E3})$$

If the number of levels  $K(\hbar)$  is irrelevant to the level spacing we identify asymptotic equidistance. In view of (E3) this poses the constraint  $\lim_{\hbar \rightarrow 0} \log K(\hbar)/\log(s_0/\hbar) = 0$ , which is equivalent to a sub-algebraic scaling of involved states, i.e.,

$$(\forall \nu > 0) \left( \lim_{\hbar \rightarrow 0} \left(\frac{\hbar}{s_0}\right)^\nu K(\hbar) = 0 \right), \quad (\text{E4})$$

since only then the  $K$ -dependent part in the denominator of Eq. (E3) becomes subdominant compared to  $\log(s_0/\hbar)$ .

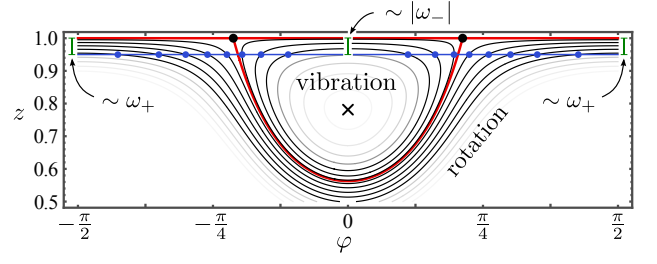

FIG. F1. Librations and rotations (black) in the vicinity of the separatrix are intersecting (blue dots) the horizontal line corresponding to the non-interacting ground state (blue solid). Non-intersecting orbits are grayed out to indicate exponentially suppressed overlaps. The criterion for intersection depends on the peak value of  $z$  located at  $\varphi = \pm \frac{\pi}{2}$  (rot.) or  $\varphi = 0$  (vib.), where  $\omega(z, \varphi)$  can be linearized in  $z$  and therefore  $1 - z = 1/(2\tilde{N}) \sim |\omega_\pm|$ .

### Appendix F: Quench dynamics of inter-particle correlations—the finite-size corrected log time

Close to criticality  $E \approx E_{\text{sep}}$ , the eigenstates of the bosonic system described by (A7) in the supercritical regime  $\alpha > 1$  are far from pure condensates with all atoms occupying the same single-particle mode. The associated inter-particle correlations can be quantified by the von Neumann entropy

$$S = -\text{Tr}(\hat{\rho} \log \hat{\rho}) \quad (\text{F1})$$

of the  $3 \times 3$  reduced one-body density matrix (ROBDM)

$$\rho_{kl} = \frac{1}{N} \langle \psi | \hat{a}_k^\dagger \hat{a}_l | \psi \rangle \quad (\text{F2})$$

of a pure  $N$ -particle state  $|\psi\rangle$ .

To study entanglement spreading as another facet of quantum information scrambling we consider (as in [16]) the evolution of  $S(t)$  after the quantum quench, where the non-interacting ground state, i.e., the pure condensate  $|\psi(t=0)\rangle = 1/\sqrt{N!}(\hat{a}_0^\dagger)^N|0\rangle$ , evolves subject to the interacting Hamiltonian (A7) with  $\alpha > 1$ . Eq. (F1) expresses inter-particle correlations as loss of information when all but one particles are traced out. An initial increase of  $S(t)$  after the quench thus represents a form of information scrambling, similar to the increase of the OTOC [Eq. (13) of the main text]: While the latter quantifies the scrambling of information among sites or modes, the former quantifies scrambling among *particles*.

Because of total momentum conservation  $[\hat{K}, \hat{\mathcal{H}}] = 0$  in the considered system, the ROBDM takes a very simple form. The time-evolved state becomes

$$|\psi(t)\rangle = \sum_{m=0}^{\frac{N}{2}} c_m(t) |m, N-2m, m\rangle \quad (\text{F3})$$

(with  $N$  even for simplicity), represented in Fock basis

$$|m_{-1}, m_0, m_1\rangle \equiv \frac{(\hat{a}_{-1}^\dagger)^{m_{-1}} (\hat{a}_0^\dagger)^{m_0} (\hat{a}_1^\dagger)^{m_1}}{\sqrt{m_{-1}! m_0! m_1!}} |0\rangle, \quad (\text{F4})$$

where  $|0\rangle$  denotes the vacuum of  $N = 0$  particles. Because the operator  $\hat{a}_k^\dagger \hat{a}_l$  cannot change three occupation numbers simultaneously, its matrix elements are restricted to

$$\langle n, N - 2n, n | \hat{a}_k^\dagger \hat{a}_l | m, N - 2m, m \rangle \propto \delta_{nm} \delta_{kl}. \quad (\text{F5})$$

This results in the diagonal form

$$\hat{\rho}(t) = \frac{1}{N} \begin{pmatrix} \langle m_{\pm 1} \rangle_t & 0 & 0 \\ 0 & N - 2\langle m_{\pm 1} \rangle_t & 0 \\ 0 & 0 & \langle m_{\pm 1} \rangle_t \end{pmatrix}, \quad (\text{F6})$$

depending only on the expectation value  $\langle m_{\pm 1} \rangle_t = \sum_m |c_m(t)|^2 m$  of the  $k = \pm 1$  momentum mode occupation.

When represented in the energy eigenbasis  $\{|n\rangle\}$  of the interacting system, the ROBDM reads

$$\rho_{kl}(t) = \frac{1}{N} \sum_{n,m} d_n^* d_m \langle n | \hat{a}_k^\dagger \hat{a}_l | m \rangle e^{-i(E_m - E_n)t}, \quad (\text{F7})$$

where  $d_n = \langle n | \psi(0) \rangle$ . States in the vicinity of the ES-QPT are dominantly involved in the process, because  $|\psi(0)\rangle$  corresponds to the classical orbit given by the horizontal line  $z = 1 - 1/(2\tilde{N})$ , very close to the upper boundary of the phase space. A semiclassical estimate of the number of states around the separatrix that are dominantly involved is given by the criterion that the corresponding orbits intersect this horizontal line as depicted in Fig. F1. This is because the overlap  $d_n$  typically drops off exponentially for states  $|n\rangle$  whose corresponding quantized orbits are beyond intersection, analogous to the exponential decay of WKB wave functions in classically forbidden regions. From a linearization of  $\omega(z, \varphi)$  at  $(z, \varphi) = (1, \pi/2)$  and  $(z, \varphi) = (1, 0)$ , valid for large  $N$ , one gets the corresponding bound  $\omega_- < \omega < \omega_+$  with  $\omega_- = -(\alpha - 1)/\tilde{N}$  and  $\omega_+ = 1/\tilde{N}$ , both scaling as  $\omega_{\pm} \sim 1/\tilde{N}$ . In view of (E1) the number of dominantly contributing states thus scales subalgebraically as

$$K \sim |\omega_{\pm}| \tilde{N} \log \tilde{N} \sim \log N, \quad (\text{F8})$$

justifying the use of (E1) in the first place and fulfilling the requirement (E4) for asymptotically constant level spacing. While for exactly equidistant energies  $E_m - E_n = (m - n)\Delta E$  the ROBDM (F7) becomes periodic in time with period  $\tau = 2\pi/\Delta E$ , this periodicity is flawed for finite  $N$ , resulting in only partial recurrence, because neither is the spectrum exactly equidistant for dominantly contributing states, nor can states with larger  $|\omega| > |\omega_{\pm}|$  be fully ignored. When increasing  $N$  the periodicity should slowly become more and more perfect. This tendency is demonstrated in figure Fig. F2.

For finite  $N$  one can estimate the correction to the characteristic time scale by averaging the inverse level spacing  $\Delta\omega^{-1} = \bar{\varrho}(\omega)$  over the interval  $\omega \in [\omega_-, \omega_+]$  assuming constant weight:

$$\langle \Delta\omega^{-1} \rangle_{\omega} = \frac{1}{\omega_+ - \omega_-} \int_{\omega_-}^{\omega_+} d\omega \bar{\varrho}(\omega) = \frac{1}{\langle \Delta\omega \rangle_n}, \quad (\text{F9})$$

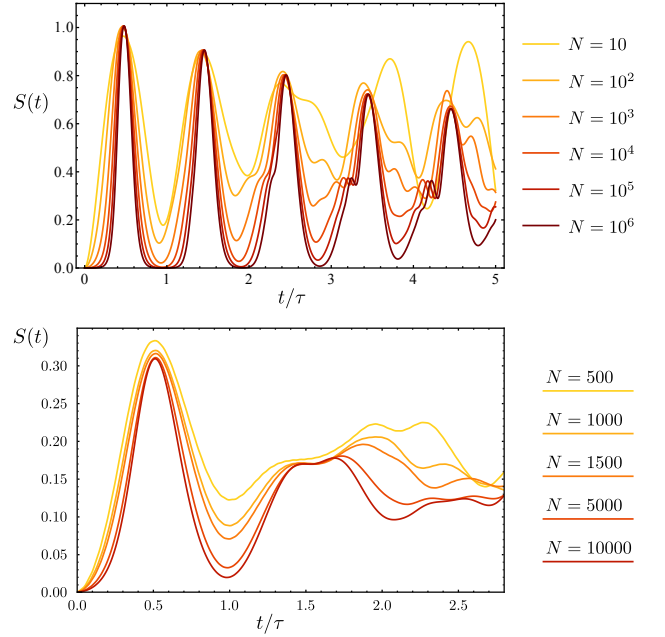

FIG. F2. Evolution of the von Neumann entropy (F1) of the ROBDM (F2) initialized in the non-interacting ground state. Upper panel: Evolution in the integrable three-mode model for  $\alpha = 2$  and  $N = 10^n$  with  $n = 1, 2, 3, 4, 5, 6$ , calculated by numerical exact diagonalization. The increasing quality of periodicity with growing  $N$  is in particular reflected in the improvement of revivals  $S(j\tau) \approx 0$  for  $j \in \mathbb{N}$ . The time is scaled with the (pseudo-)period  $\tau$  (F10) associated with the estimate for the average involved level spacing. Lower panel: Evolution in the non-integrable five-mode model for  $\alpha = 1.05$  and  $N = 500, 1000, 1500, 5000, 10000$ , calculated numerically in a converged adiabatic expansion (see App. G). Although non-integrable, the dynamics shows the same tendency towards revivals, where the (pseudo-)period  $\tau$  is again of log type [see Eq. (12) of the main text] with  $\lambda \approx 0.21$  coinciding with the dynamical instability  $\lambda_s \approx 2\lambda$  in the corresponding classical phase space.

which coincides with the inverse arithmetic mean of all involved spacings  $\Delta\omega$  and results in the estimated time scale

$$\tau = \frac{1}{\sqrt{\alpha - 1}} \left[ \log N + 1 + \log \left( \frac{128(\alpha - 1)^2}{\alpha^2(8 - \alpha)} \right) - \frac{\alpha - 1}{\alpha} \log(\alpha - 1) \right]. \quad (\text{F10})$$

Since (F10) is the characteristic time scale of the whole evolution of  $S(t)$ , it directly determines the scrambling time  $\tau_{\text{scr}}$ , which refers to the initial growth. Defined by the condition  $S(\tau_{\text{scr}}) = S_{\text{th}}$  with some arbitrary, small valued threshold entropy  $S_{\text{th}}$ , the scrambling time asymptotically becomes

$$\tau_{\text{scr}} = \text{const.} \times \frac{1}{\sqrt{\alpha - 1}} \log N + \mathcal{O}(1). \quad (\text{F11})$$

The logarithmic scaling with  $N$  as a numerical observation has already been reported in Ref. [16], where

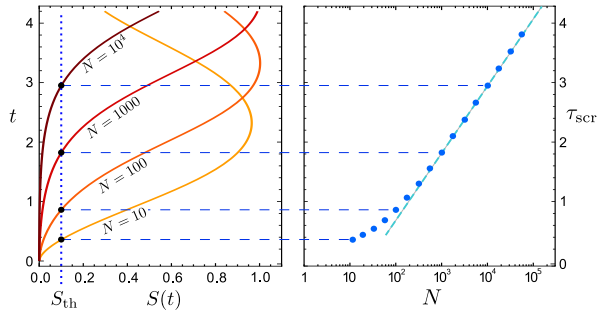

FIG. F3. Scrambling times  $\tau_{\text{scr}}$  for  $\alpha = 2$  obtained from numerically evolved entropies  $S(t)$  (F1) using the threshold  $S_{\text{th}} = 0.1$  for several numbers of particles (left). Plotting those against  $N$  logarithmically (right) shows a linear dependence on  $\log N$  for  $N \gtrsim 100$ , confirming the scaling in Eq. (F11). The prefactor and additive constant are fitted (dashed).

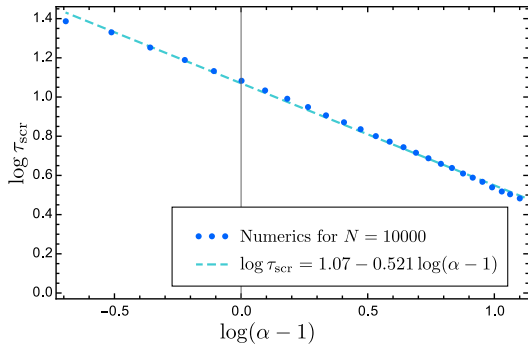

FIG. F4. Numerical scrambling times obtained as in Fig. F3 for  $N = 10^4$  as a function of  $\alpha$ . A linear fit to the doubly logarithmic data supports the predicted dominant scaling with  $\sqrt{\alpha - 1}$  (F11). Deviations thereof (small mismatch in the exponent 0.521 from the prediction 0.5 and additional functional dependence on  $\alpha$ ) are attributed to finite-size effects expected to vanish asymptotically.

also a general connection to an instability has been suspected. The semiclassical treatment presented here provides sufficient analytical ground for supplying those statements with explicit analytical expressions and thorough derivation. Furthermore, the one-to-one correspondence between  $S(t)$  and the mean condensate fraction  $\langle \psi | \hat{n}_0(t) | \psi \rangle / N$ , as evident from (F6), establishes a connection to Ref. [17], where oscillatory behavior has been reported based on a quasi-classical picture valid for times up to  $\tau_E$ . While the classical phase space sampling used in [17] infers decaying oscillations of  $S(t)$ , unitary quantum evolution, implemented in our approach (10), implies strong revivals, periodically leading to  $S(t) \approx 0$  beyond  $\tau_E$ . Eventually, for  $N \rightarrow \infty$ , the quantum and quasi-classical picture become unified again, due to the peculiarity of asymptotic spectral equidistance, analogous to harmonic oscillator levels, where a quasi-classical description would become exact. Finally, Figs. F3 and F4 show numerical confirmation of (F11).

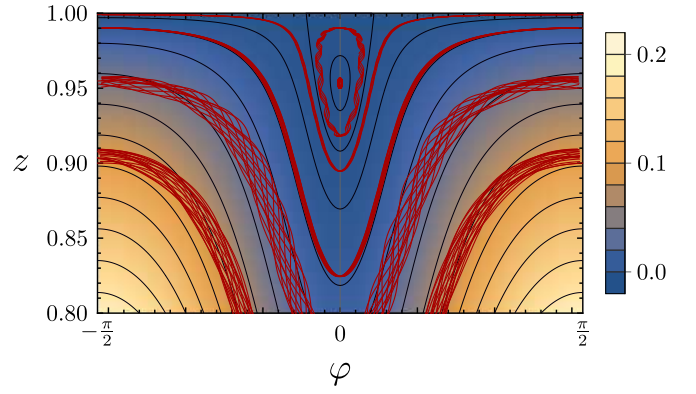

FIG. G1. Effective mean-field phase space portrait obtained from minimizing the fast degrees of freedom (density and black contours). The red curves show the projections of the full dynamics (initialized close to the respective manifolds) to the slow degrees of freedom  $(\varphi, z)$ .

## Appendix G: Extension to five modes

To verify the existence of a unique log time scale in a more general setup we have investigated the attractive Lieb-Liniger model in 5-mode approximation by including the  $k = \pm 2$  single-particle momentum modes in Eq. (3) of the main text. As in the 3-mode approximation, the total momentum and particle number are conserved quantities such that one can restrict to the sector of Fock space with fixed total momentum  $K$  ( $K = 0$  in the following) and particle number  $N$ . In addition, for  $K = 0$ , the states can be chosen to be eigenstates of the parity operator that inverts the sign of the single-particle momentum. The basis size of the respective sector will then scale as  $N^3$  in contrast to the linear scaling in the 3-mode approximation. Therefore, to obtain numerical results for large particle numbers one has to make use of further approximations. A key observation is the fact that the low-lying spectrum around criticality is composed of different kinds of excitations that motivate a separation of the dynamics into fast and slow degrees of freedom, the latter being given by the condensate fraction. This observation was verified using the classical limit of the 5-mode approximated Hamiltonian in the spirit of App. B. After eliminating the classical constants of motion corresponding to the total particle number and the total momentum an effective 1D mean field description can be found by fixing the classical variable that corresponds to the condensate fraction as well as its canonical conjugate phase and minimizing the energy with respect to the other (fast) phase space variables (see Fig. G1). Close to the mean-field critical point the dynamics of the trajectories at low energies are well approximated within this effective description, as demonstrated in Fig. G1. This justifies the adiabatic separation that should become better with larger particle numbers, as the level spacings between the excitations corresponding to slow degrees of freedom decrease faster

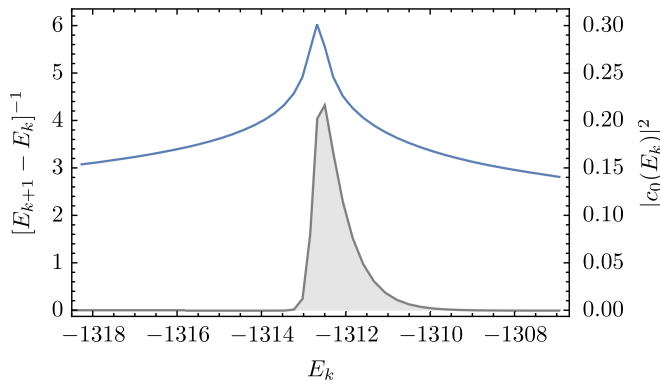

FIG. G2. Inverse level spacing within the first band for  $N = 5000$ ,  $\alpha = 1.05$ . As in the 3-mode approximation a logarithmic peak in the density of states forms (blue, solid). The gray shaded plot shows the squared overlaps of the respective states with the initial state, i.e., the noninteracting ground state.

with the particle number as compared to the excitations corresponding to the fast degrees of freedom. The effective 1D phase space portrait is a deformed version of the phase space of the 3-mode model with two hyperbolic fixed points at the upper boundaries for  $\alpha > 1$ . Their stability exponents have been calculated numerically as  $\lambda_s \approx 0.42$  for  $\alpha = 1.05$ .

The adiabatically decoupled subspectra are also observed numerically (distinguishable, e.g., by comparing mean occupations of the  $k = \pm 2$  modes in the quantum states). As a major result, the individual subspectra have a regular level spacing as expected from 1D systems, with a peak in the density of states at the energy of the separatrix of the effective phase space. This is demonstrated in Fig. G2, where the inverse level spacing within the lowest subspectrum is shown. Moreover, the noninteracting condensate overlaps dominantly with states within this peak (shaded curve in Fig. G2), indicating that the quench dynamics is dominated by only a few states around an excited state quantum phase transition with level spacings that we expect to be asymptotically equidistant.

To implement the adiabatic separation on a quantum-mechanical level, simply replacing the creation and annihilation operators corresponding to the zero mode by complex variables leads to a  $U(1)$ -symmetry-broken effective description for the fast degrees of freedom with an infinite-dimensional Hilbert space, rendering this approach not suitable for numerical diagonalization. We have chosen a different approach that consists of a prediagonalization of the restrictions of the Hamiltonian to subspaces with a fixed mean condensate fraction  $\bar{z} = \bar{n}_0/N$ . In particular, a “good” basis is found using the subspaces  $\mathcal{R}_k = \mathcal{H}_{2k-1} \oplus \mathcal{H}_{2k}$  with  $k = 1, \dots, N/2$ , where  $\mathcal{H}_n = \{|\psi\rangle \in \mathcal{H} : \hat{a}_0^\dagger \hat{a}_0 |\psi\rangle = n |\psi\rangle\}$  is the subspace with fixed particle number  $N$ , total momentum  $K = 0$  and zero-mode occupation  $n$ . The dimension of the space

| $N$               | 100 | 500 | 1000 | 1500 | 5000 | 10000 |
|-------------------|-----|-----|------|------|------|-------|
| $\zeta$           | 40  | 100 | 200  | 300  | 1000 | 2000  |
| $\Delta_2^{\max}$ | 20  | 30  | 20   | 30   | 50   | 50    |
| $\Sigma_2^{\max}$ | 40  | 60  | 40   | 60   | 100  | 100   |

TABLE I. Cutoffs that were used in the numerical calculations.

$\mathcal{R}_k$  scales as  $(N - 2k)^2$ , such that the restrictions of the Hamiltonian to  $\mathcal{R}_k$  can be effectively diagonalized for large particle numbers, yielding a  $k$ -dependent eigenbasis  $\{v_\nu^{(k)} : \nu = 0, 1, \dots\}$  (ordered by energy) that spans  $\mathcal{R}_k$ . The space  $\text{span}(\{v_\nu^{(k)} : k = 0, 1, \dots\})$  may then be referred to as the  $\nu$ -th band. An effective Hamiltonian is found by restricting the full Hamiltonian to the space

$$\mathcal{S}_\eta^\zeta = \bigoplus_{k=1}^{\zeta} \text{span}(\{v_\nu^{(k)} : \nu \leq \eta\}), \quad (\text{G1})$$

where we introduced a cutoff  $2\zeta \leq N$  in the condensate depletion as well as a cutoff  $\eta$  controlling the number of excitations in the fast degrees of freedom taken into account via inter-band coupling. It turns out that already for  $\eta = 0$ , where the effective Hamiltonian has the same structure as for the 3-mode approximation, the lowlying excitation spectrum around the critical point  $\alpha = 1$  is well described. For our numerical calculations of the vectors  $v_\nu^{(k)}$  we introduced two further cutoffs  $\Sigma_2 = n_2 + n_{-2} \leq \Sigma_2^{\max}$ ,  $\Delta_2 = |n_2 - n_{-2}| \leq \Delta_2^{\max}$ , where  $n_2, n_{-2}$  are the occupations of the  $\pm 2$  single-particle momentum modes. All cutoffs have been varied to check the convergence of the results. The data presented in Fig. 5(b) of the main text and Fig. F2 uses the cutoffs shown in table I, where  $\eta = 80$  for all the values of  $N$ . The time evolution was approximated using the first 2000 eigenstates of the effective Hamiltonian matrix for particle numbers  $N \geq 500$  (for  $N = 100$  all eigenstates were used). The convergence of the results with respect to this approximation has been checked, again, by varying the number of eigenstates.

- 
- [1] Y. Castin, *J. Phys. IV France* **116**, 89 (2004).
  - [2] E. H. Lieb and W. Liniger, *Phys. Rev.* **130**, 1605 (1963).
  - [3] M. Olshanii, *Phys. Rev. Lett.* **81**, 938 (1998).
  - [4] Y. Nishida, *Phys. Rev. A* **97**, 061603 (2018).
  - [5] L. Pricoupenko, *Phys. Rev. A* **97**, 061604 (2018).
  - [6] G. Guijarro, A. Pricoupenko, G. E. Astrakharchik, J. Boronat, and D. S. Petrov, *Phys. Rev. A* **97**, 061605 (2018).
  - [7] R. Kanamoto, H. Saito, and M. Ueda, *Phys. Rev. Lett.* **94**, 090404 (2005).
  - [8] R. Kanamoto, H. Saito, and M. Ueda, *Phys. Rev. A* **73**, 033611 (2006).
  - [9] A. G. Sykes, P. D. Drummond, and M. J. Davis, *Phys. Rev. A* **76**, 063620 (2007).
  - [10] C. Gardiner and P. Zoller, *Quantum Noise: A Handbook of Markovian and Non-Markovian Quantum Stochastic Methods with Applications to Quantum Optics*, Springer Series in Synergetics (Springer Berlin, 2004).
  - [11] Q. Hummel, *Semiclassical Theory of Few- and Many-body Quantum Systems with Short-range Interactions*, *Ph.D. thesis*, Universität Regensburg (2018).
  - [12] L. Pitaevskii and S. Stringari, *Bose-Einstein Condensation and Superfluidity*, International Series of Monographs on Physics (Oxford University Press, 2016).
  - [13] R. M. Corless, G. H. Gonnet, D. E. G. Hare, D. J. Jeffrey, and D. E. Knuth, *Adv. Comput. Math.* **5**, 329 (1996).
  - [14] P. Stránský, M. Macek, and P. Cejnar, *Ann. Phys.* **345**, 73 (2014).
  - [15] M. A. Caprio, P. Cejnar, and F. Iachello, *Ann. Phys.* **323**, 1106 (2008).
  - [16] G. Dvali, D. Flassig, C. Gomez, A. Pritzel, and N. Wintergerst, *Phys. Rev. D* **88**, 124041 (2013).
  - [17] R. Mathew and E. Tiesinga, *Phys. Rev. A* **96**, 013604 (2017).
